# Supplementary material for: Graduated Optimization of Black-Box Functions
Source: arXiv:1906.01279 source file (2019-06-04)
Supplement: Supplementary file 1 [file appendix.tex]

\section{}
\begin{table}[h!]
\begin{small}
\bgroup
%  1 is the default, change whatever you need
\begin{tabular}{l | l | c}
\hline 
\textbf{Problem} & \textbf{Objective Function} & \textbf{Domain} \\
\hline 
Auto MPG & 
\multirow{5}{*}{
	\bgroup
	%  1 is the default, change whatever you need
	\begin{tabular}[c]{@{}l@{}}
		$\frac{1}{10}\sum_{k=1}^{10} 1 - \frac{\sum_{i\in D_k}(\hat{f}_k(X_i)-Y_i)^2}{\sum_{i\in D_k}(\overline{Y}-Y_i)^2}$, \\
		where: \\
			\hspace{0.4cm} $\hat{f}_k \in \argmin_{f \in \mathcal{H}_{\sigma}} \frac{1}{n- |D_k|} \sum_{i \not\in D_k}(f(X_i)-Y_i)^2 + \lambda \|f\|_{\mathcal{H}_{\sigma}} $, \\
			\hspace{0.4cm} the data set $\{(X_i, Y_i)\}_{i=1}^n$ is split into 10 folds $D_1, ...D_{10}$,  \\
			\hspace{0.4cm} $\mathcal{H}_{\sigma}$ denotes the gaussian RKHS of bandwidth $\sigma$, \\
			\hspace{0.4cm} $\|f\|_{\mathcal{H}_{\sigma}}$ is the corresponding norm, \\
			\hspace{0.4cm} $\sigma = 10^{x_0}, \lambda = 10^{x_1}$ \\
	\end{tabular}
	\egroup
} &
\multirow{5}{*}{$[-2,4]\times[-5,5]$} \\
Breast Cancer			&			& \\
Concrete (Slump)	&			& \\
Yacht 						& 		& \\
Housing 					& 		& \\
\hline 
Auto MPG HD & 
\multirow{5}{*}{
	\bgroup
	%  1 is the default, change whatever you need
	\begin{tabular}[c]{@{}l@{}}
		$\frac{1}{10}\sum_{k=1}^{10} 1 - \frac{\sum_{i\in D_k}(\hat{f}_k(X_i)-Y_i)^2}{\sum_{i\in D_k}(\overline{Y}-Y_i)^2}$, \\
		where: \\
			\hspace{0.4cm} $\hat{f}_k \in \argmin_{f \in \mathcal{H}_{\sigma}} \frac{1}{n- |D_k|} \sum_{i \not\in D_k}w_i(f(X_i)-Y_i)^2 + \lambda \|f\|_{\mathcal{H}_{\sigma}} $, \\
			\hspace{0.4cm} the data set $\{(X_i, Y_i)\}_{i=1}^n$ is split into 10 folds $D_1, ...D_{10}$,  \\
			\hspace{0.4cm} $\mathcal{H}_{\sigma}$ denotes the gaussian RKHS of bandwidth $\sigma$, \\
			\hspace{0.4cm} $\|f\|_{\mathcal{H}_{\sigma}}$ is the corresponding norm, \\
			\hspace{0.4cm} $\sigma = 10^{x_0}, \lambda = 10^{x_1}$ \\
	\end{tabular}
	\egroup
} &
\multirow{5}{*}{
	\bgroup
	\begin{tabular}{c}
		$[-2,4]\times[-5,5]$\\
		$\times[0,1]^n$ \\
	\end{tabular}
	\egroup
} \\
Breast Cancer HD			&			& \\
Concrete (Slump) HD	&			& \\
Yacht HD 						& 		& \\
Housing HD					& 		& \\

\end{tabular}
\caption{Details of the problems in the benchmark used for evaluations}
\label{tab:appendix_problem_functions}
\egroup
\end{small}
\end{table}
%\captionof{Table X:}{Description of the test functions of the benchmark, based on \cite{malherbe2017global}}

%\end{landscape}
